# Supplementary material for: Resilient-Economic Coordinated Robust Operation of Integrated Electric-Gas Systems
Source: arXiv:2304.14909 source file (2023-05-01)
Supplement: Supplementary file 2 [file AppendixC.tex]

\chapter{Algorithms Data} % Main appendix title

\label{AppendixB} % For referencing this appendix elsewhere, use \ref{AppendixA}

\section{Gas flow Correction Algorithm}

\section{The S-MISOCP Algorithm}

\section{The C\&CG Algorithm}

\section{The P-MICCP Algorithm}

\section{The SPP Algorithm}

\section{The BRD Algorithm}
