# Supplementary material for: Resilient-Economic Coordinated Robust Operation of Integrated Electric-Gas Systems
Source: arXiv:2304.14909 source file (2023-05-01)
Supplement: Supplementary file 3 [file AppendixTemplate.tex]

% Appendix Template

\chapter{Appendix Title Here} % Main appendix title

\label{AppendixX} % Change X to a consecutive letter; for referencing this appendix elsewhere, use \ref{AppendixX}

Write your Appendix content here.
